# Supplementary material for: A joint Bayesian hierarchical model for estimating SARS-CoV-2 diagnostic and subgenomic RNA viral dynamics and seroconversion
Source: arXiv:2301.03714 ancillary file (2023-01-09)
Supplement: Supplementary file 1 [file Supplement_cohort2.pdf]

# Supplementary materials for "A joint Bayesian hierarchical model for estimating SARS-CoV-2 diagnostic and subgenomic RNA viral dynamics and seroconversion"

Tracy Q. Dong[1] and Elizabeth R. Brown[1,2]

[1] Vaccine and Infectious Disease Division, Fred Hutchinson Cancer Research Center

[2] Department of Biostatistics, University of Washington

January 9, 2023

## S1 COVID-19 PEP study - model implementation details

### S1.1 Prior specification

Based on Kissler et al. (2021a,b), and Stankiewicz Karita et al. (2021), we specified the following priors for the model parameters representing diagnostic RNA viral load characteristics:

$$\mu_{lvp} \sim \text{Normal}\left(\text{mean} = \log(5), \text{sd} = 0.2\right),$$
$$\mu_{lwa} \sim \text{Normal}\left(\text{mean} = \log(2), \text{sd} = 0.2\right),$$
$$\mu_{lwb} \sim \text{Normal}\left(\text{mean} = \log(9), \text{sd} = 0.2\right).$$

Based on Deming et al. (2022), the following priors were used for the sgRNA viral load characteristics:

$$\mu_{td} \sim \text{Normal}\left(\text{mean} = 0, \text{sd} = 1\right)$$
$$\mu_{lwd} \sim \text{Normal}\left(\text{mean} = \log(5), \text{sd} = 0.2\right),$$
$$\gamma_1 \sim \text{Gamma}\left(\text{shape} = 20, \text{rate} = 1\right),$$
$$\gamma_2 \sim \text{Gamma}\left(\text{shape} = 10, \text{rate} = 1\right).$$

For the parameters characterising the true positive rate (TPR) and true negative rate (TNR) of the diagnostics and sgRNA viral load samples, we use the following priors:

$$\alpha_0 \sim \text{Normal}\left(\text{mean} = -4, \text{sd} = 0.2\right),$$
$$\alpha_1 \sim \text{Normal}\left(\text{mean} = 8, \text{sd} = 0.2\right),$$
$$\alpha_0' \sim \text{Normal}\left(\text{mean} = -4, \text{sd} = 0.2\right),$$
$$\alpha_1' \sim \text{Normal}\left(\text{mean} = 8, \text{sd} = 0.2\right).$$

We used weakly informative priors for all coefficient parameters:

$$\boldsymbol{\beta}_{vp}[j] \sim \text{Normal}\left(\text{mean} = 0, \text{sd} = 0.5\right) \quad \text{for all } j,$$
$$\boldsymbol{\beta}_{C}[k] \sim \text{Normal}\left(\text{mean} = 0, \text{sd} = 0.5\right) \quad \text{for all } k.$$

Similarly, we used weakly informative priors for all variance parameters:

$$\sigma_{yy} \sim \text{T}\left(df = 30\right),$$
$$\sigma_{yy}' \sim \text{T}\left(df = 30\right),$$
$$\boldsymbol{\Sigma}_{log} \sim \text{Inv.Wishart}\left(\boldsymbol{I}_3, df = 20\right).$$

where $\boldsymbol{I}_3$ is an identity matrix of 3 rows.

Finally, we specify the following priors for the parameters quantifying extra variability in viral load measurements below LoQ and the Gamma distribution for the seroconversion time since infection:

$$\delta_Q \sim \text{Beta}\left(10, 30\right),$$
$$\kappa_1 \sim \text{Gamma}\left(\text{shape} = 50, \text{rate} = 2\right),$$
$$\kappa_2 \sim \text{Gamma}\left(\text{shape} = 20, \text{rate} = 10\right).$$

## S1.2 Markov Chain Monte Carlo (MCMC) setup

All models were implemented in R 4.2.1 (R Core Team, 2022) using JAGS 4.3.0 (Plummer et al., 2003). For each model, we performed the adaptation phase for 10000 iterations and ran 2 independent MCMC chains. Each chain was run for a total of 40000 iterations: the first 20000 were discarded as burn-in and the remaining 20000 were thinned to 1/10 of the iterations (i.e., 2000) saved for inference.

## S1.3 Model diagnostics

For model diagnostics, we examined the following plots and summary metrics for key model parameters:

- Histograms of posterior samples.
- Density plots with different colors by chain.
- Traceplots with different colors by chain to assess convergence and chain problems.
- Plots of the running means to check how quickly the chain is approaching its target distribution.
- Overlapped density plots that compare the last 10 percent of the chain with the whole chain.
- Autocorrelation plots to check for autocorrelation of posterior samples.
- Crosscorrelation plot to diagnose potential problems of convergence due to highly correlated parameters.
- The Potential Scale Reduction Factor ($\hat{R}$)(Gelman et al., 2013) for comparison of the between-chain variation with the within-chain variation.
- The Geweke z-score diagnostic (Geweke, 1992) for comparison of the first part of the chain with its last part.

The ggmcmc package in R was used to create model diagnostics for each model fitted. The full diagnostic report for our primary model can be found online at https://github.com/dq0708/joint_vl_sero.

## S2 Supplemental tables

| Type | Parameter | Mean | SD | Percentile | | |
|---|---|---|---|---|---|---|
| | | | | 2.5% | 50% (Median) | 97.5% |
| Diagnostic RNA | $\mathbf{\Sigma}_{log}[1,1]$ | 0.07 | 0.01 | 0.05 | 0.07 | 0.10 |
| viral load | $\mathbf{\Sigma}_{log}[2,2]$ | 0.58 | 0.14 | 0.36 | 0.56 | 0.91 |
| | $\mathbf{\Sigma}_{log}[3,3]$ | 0.14 | 0.03 | 0.10 | 0.14 | 0.20 |
| | $\mathbf{\Sigma}_{log}[1,2]$ | 0.02 | 0.03 | -0.05 | 0.02 | 0.09 |
| | $\mathbf{\Sigma}_{log}[1,3]$ | -0.02 | 0.01 | -0.04 | -0.02 | 0.01 |
| | $\mathbf{\Sigma}_{log}[2,3]$ | 0.03 | 0.04 | -0.05 | 0.03 | 0.11 |
| | $\sigma_{yy}$ | 0.94 | 0.03 | 0.88 | 0.94 | 1.00 |
| | $\delta_Q$ | 0.25 | 0.06 | 0.13 | 0.24 | 0.38 |
| | $\alpha_0$ | -5.27 | 0.12 | -5.52 | -5.27 | -5.03 |
| | $\alpha_1$ | 7.70 | 0.09 | 7.51 | 7.70 | 7.87 |
| | SD of $v_{p,i}$ | 1.45 | 0.09 | 1.27 | 1.44 | 1.64 |
| | SD of $w_{a,i}$ | 3.39 | 0.94 | 2.42 | 3.18 | 5.54 |
| | SD of $w_{b,i}$ | 3.93 | 0.39 | 3.39 | 3.86 | 4.90 |
| sgRNA | Mean of $q_i$ | 0.65 | 0.02 | 0.62 | 0.65 | 0.69 |
| viral load | Mean of $t'_{d,i}$ | 0.58 | 0.13 | 0.32 | 0.58 | 0.84 |
| | Mean of $w'_{d,i}$ | 4.29 | 0.15 | 4.01 | 4.28 | 4.59 |
| | SD of $q_i$ | 0.08 | 0.01 | 0.06 | 0.08 | 0.09 |
| | SD of $t'_{d,i}$ | 0.65 | 0.05 | 0.55 | 0.65 | 0.75 |
| | SD of $w'_{d,i}$ | 2.90 | 0.19 | 2.65 | 2.86 | 3.39 |
| | SD of $v'_{p,i}$ | 1.07 | 0.07 | 0.94 | 1.07 | 1.21 |
| | SD of $w'_{a,i}$ | 3.47 | 0.92 | 2.51 | 3.27 | 5.64 |
| | SD of $w'_{b,i}$ | 3.55 | 0.40 | 3.01 | 3.47 | 4.54 |
| | $\sigma'_{yy}$ | 0.82 | 0.04 | 0.75 | 0.82 | 0.89 |
| | $\alpha'_0$ | -5.48 | 0.13 | -5.73 | -5.48 | -5.22 |
| | $\alpha'_1$ | 7.64 | 0.09 | 7.46 | 7.64 | 7.81 |
| Seroconversion | $\boldsymbol{\beta}_C[1]$ — intercept | 0.01 | 0.49 | -0.93 | 0.01 | 0.98 |
| | $\boldsymbol{\beta}_C[2]$ — $v_p$ | 0.21 | 0.11 | -0.01 | 0.20 | 0.43 |
| | SD of $C_i$ | 0.43 | 0.04 | 0.36 | 0.44 | 0.49 |
| | $\kappa_1$ | 25.36 | 3.09 | 19.76 | 25.26 | 31.73 |
| | $\kappa_2$ | 1.76 | 0.23 | 1.34 | 1.76 | 2.23 |

Table S1: The posterior mean, standard deviation (SD), and 2.5%, 50% and 97.5% percentiles of key parameters in the primary joint model described in Section 4.1 of the main manuscript.

## S3 Supplemental figures

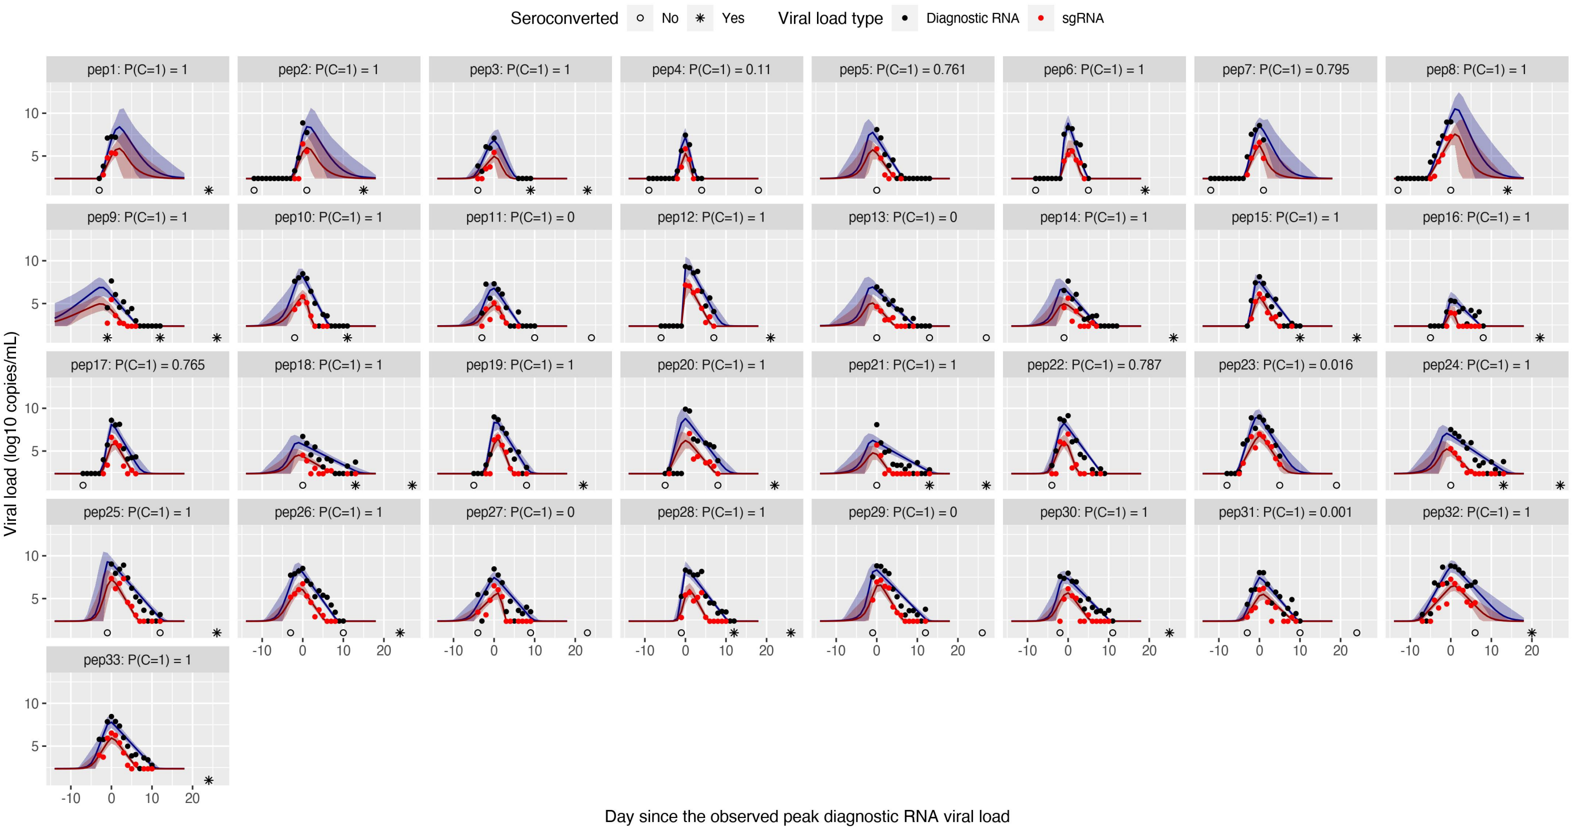


Figure S1: The observed and estimated SARS-CoV-2 diagnostic and subgenomic RNA (sgRNA) viral load trajectories and seroconversion time and probability for each individual in the COVID-19 post-exposure prophylaxis (PEP) study who had at least 2 positive sgRNA samples during the first 14 days of follow-up and had at least 1 dried blood spot (DBS) sample with confirmed results. Specifically, the diagnostic and sgRNA viral load were represented using navy and red colors respectively. The posterior means and 95% credible intervals (CIs) of the viral load trajectories were shown using lines and ribbons respectively. The posterior probability of seroconversion (i.e., $Pr(C = 1)$) is shown in the title of each panel. The observed viral load data was shown using solid dots. The observed seroconversion data was shown using circles and stars.

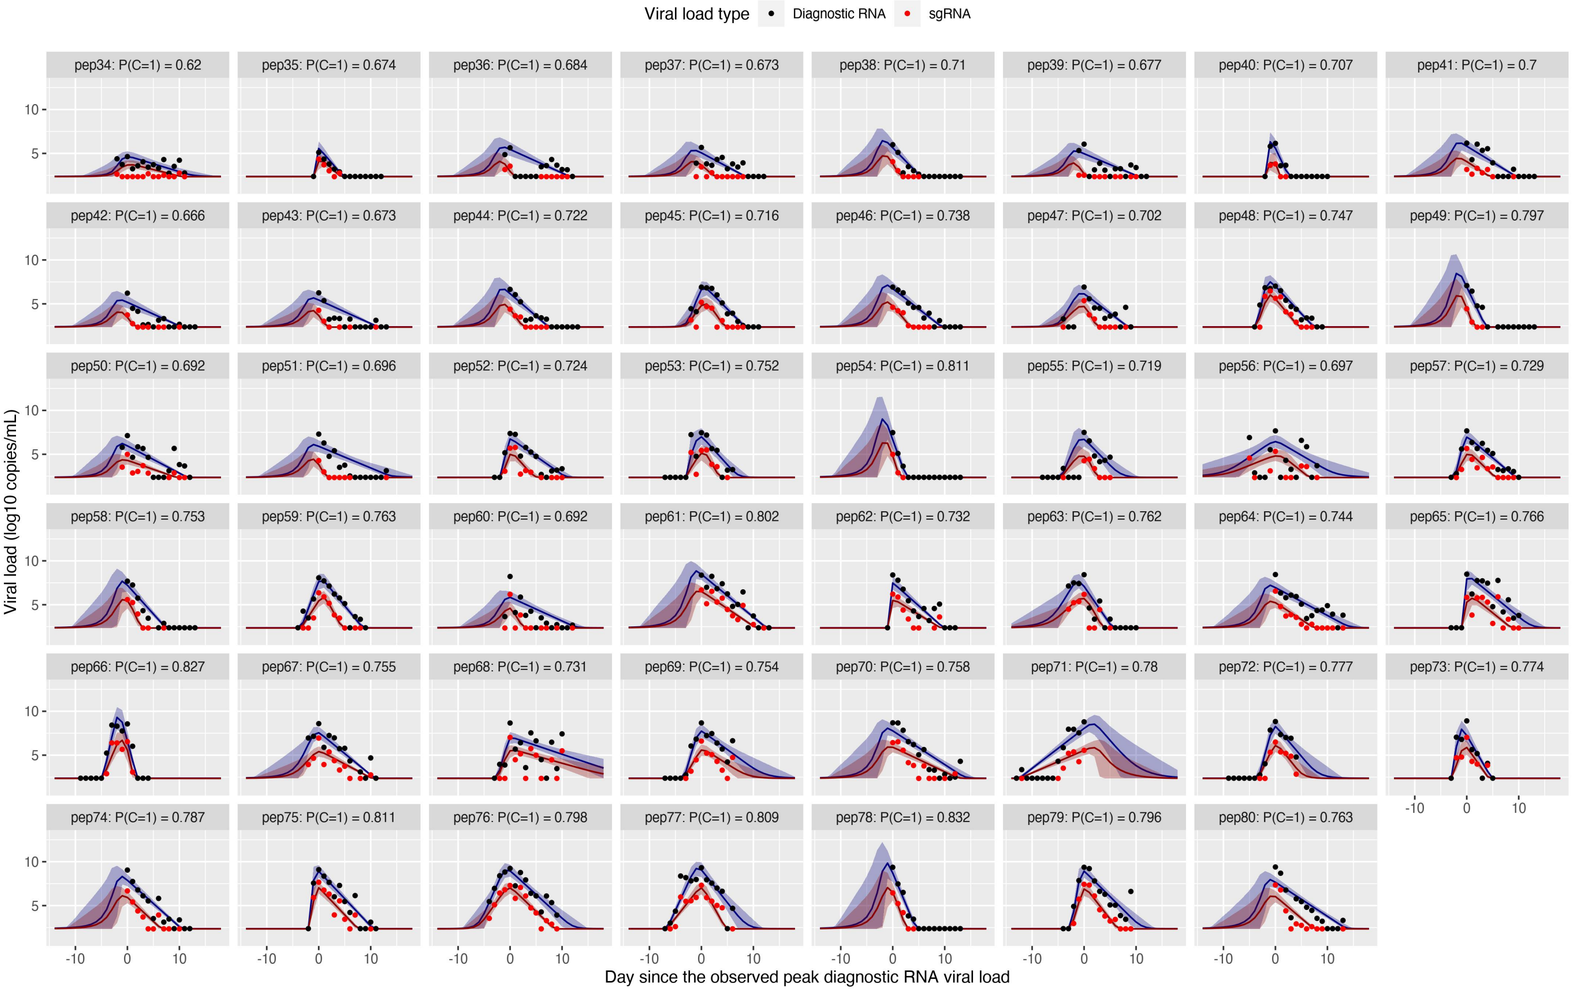


Figure S2: The observed and estimated SARS-CoV-2 diagnostic and subgenomic RNA (sgRNA) viral load trajectories and seroconversion time and probability for each individual in the COVID-19 post-exposure prophylaxis (PEP) study who had at least 2 positive sgRNA samples during the first 14 days of follow-up but no dried blood spot (DBS) sample with confirmed results. Specifically, the diagnostic and sgRNA viral load were represented using navy and red colors respectively. The posterior means and 95% credible intervals (CIs) of the viral load trajectories were shown using lines and ribbons respectively. The posterior probability of seroconversion (i.e., $Pr(C = 1)$) is shown in the title of each panel. The observed viral load data was shown using solid dots.

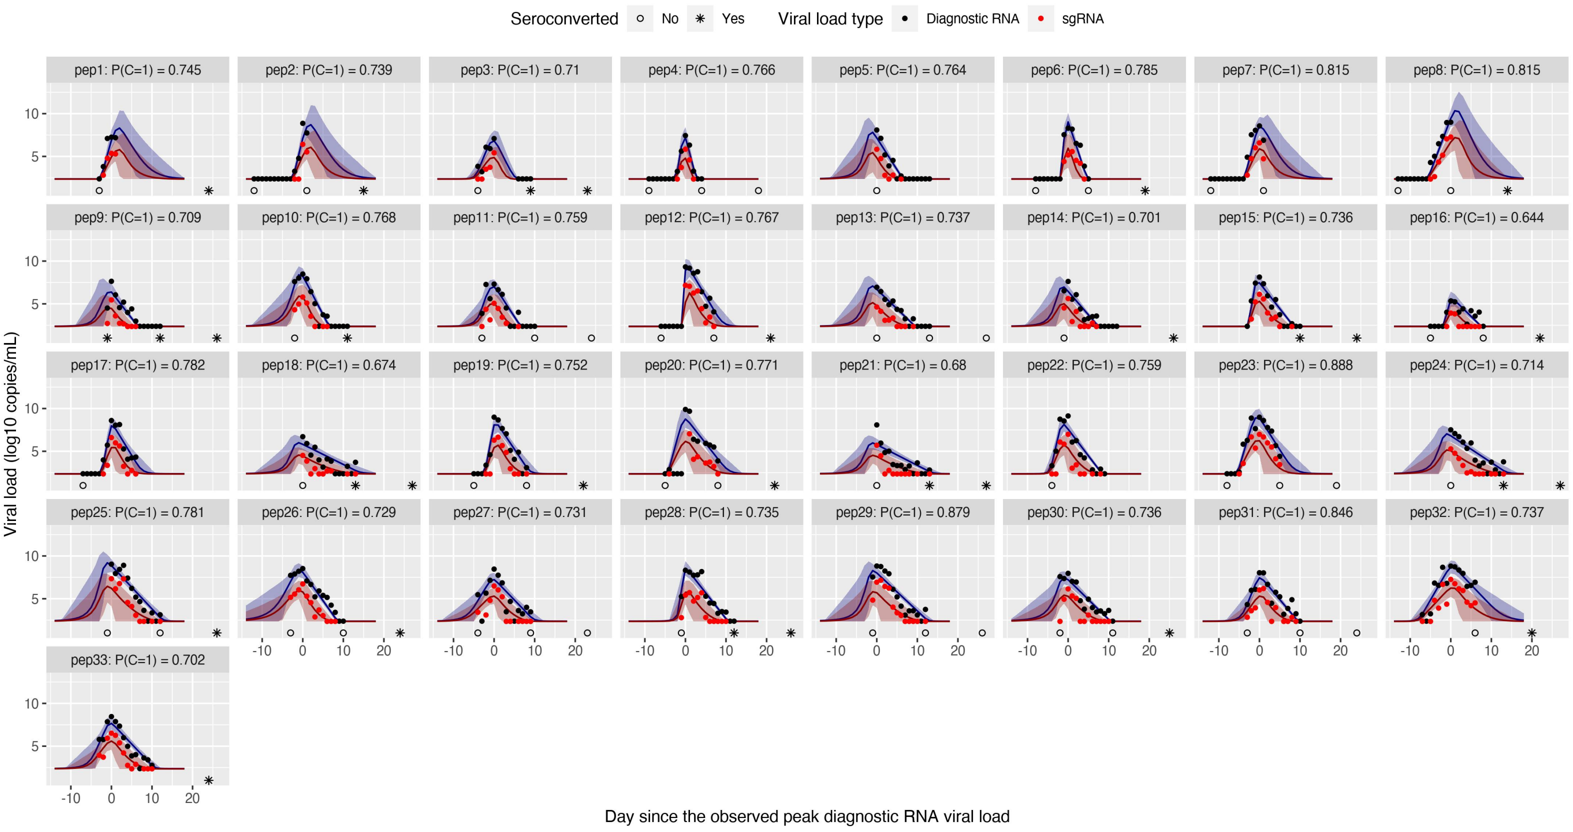


Figure S3: The observed and estimated/imputed SARS-CoV-2 diagnostic and subgenomic RNA (sgRNA) viral load trajectories and seroconversion time and probability from the 10-fold cross-validation exercise for each individual in the COVID-19 post-exposure prophylaxis (PEP) study who had at least 2 positive sgRNA samples during the first 14 days of follow-up and had at least 1 dried blood spot (DBS) sample with confirmed results. Specifically, the diagnostic and sgRNA viral load were represented using navy and red colors respectively. The posterior means and 95% credible intervals (CIs) of the viral load trajectories were shown using lines and ribbons respectively. The posterior probability of seroconversion (i.e., $Pr(C = 1)$) is shown in the title of each panel. The observed viral load data was shown using solid dots. The observed seroconversion data was shown using circles and stars.

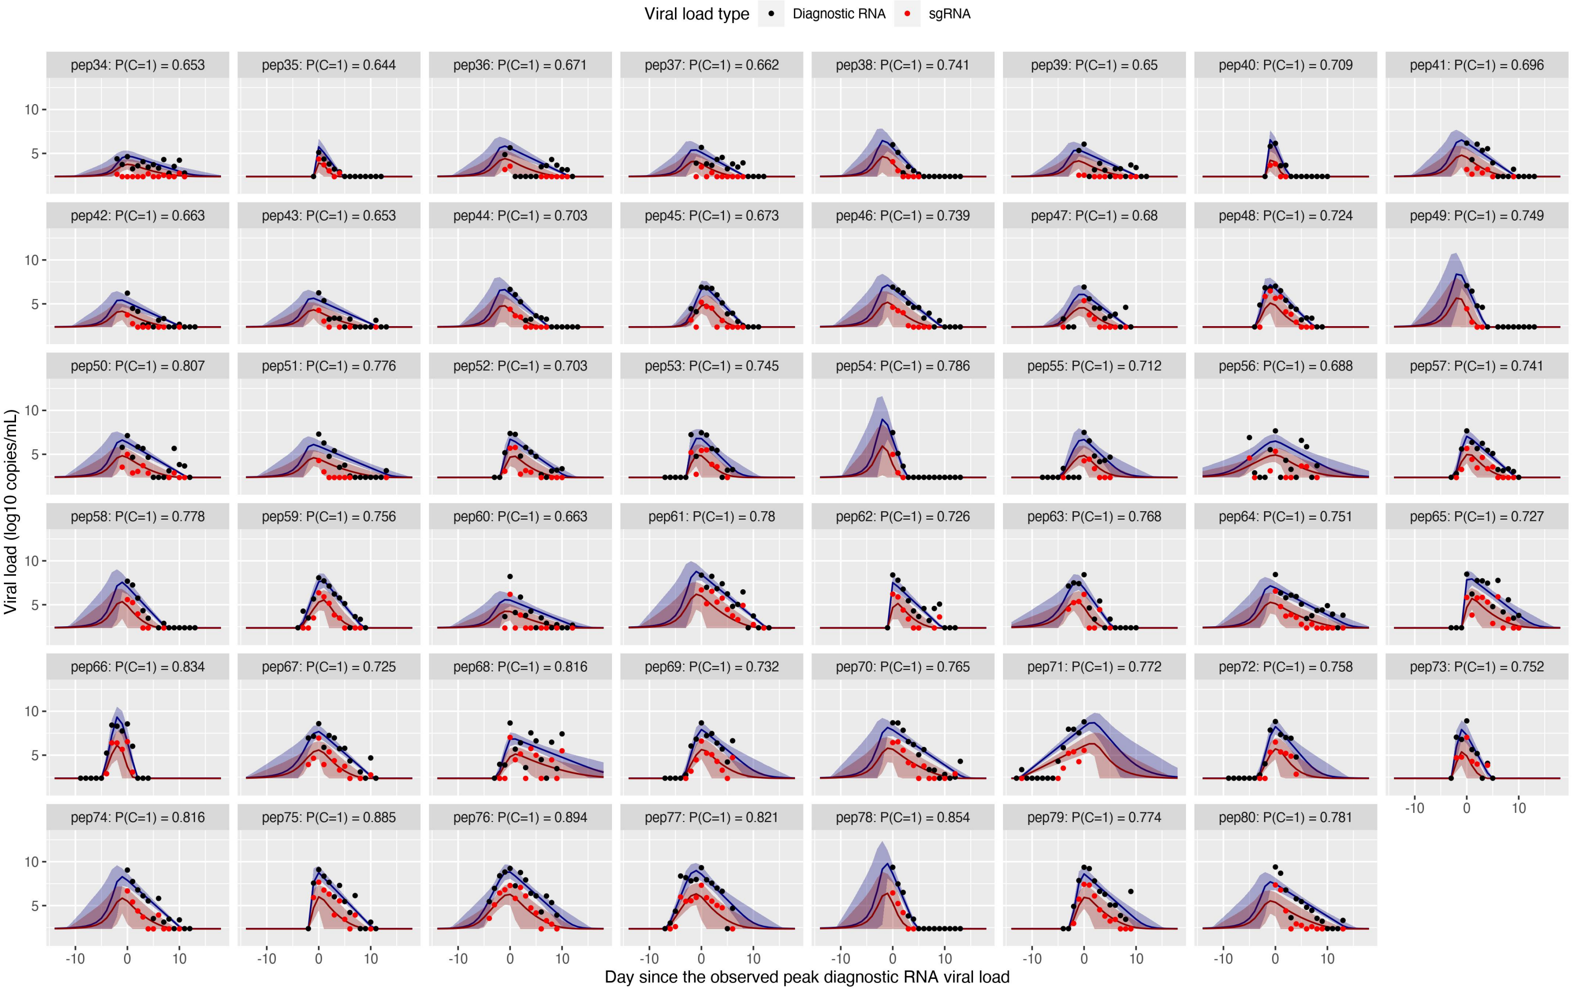


Figure S4: The observed and estimated/imputed SARS-CoV-2 diagnostic and subgenomic RNA (sgRNA) viral load trajectories and seroconversion time and probability from the 10-fold cross-validation exercise for each individual in the COVID-19 post-exposure prophylaxis (PEP) study who had at least 2 positive sgRNA samples during the first 14 days of follow-up but no dried blood spot (DBS) sample with confirmed results. Specifically, the diagnostic and sgRNA viral load were represented using navy and red colors respectively. The posterior means and 95% credible intervals (CIs) of the viral load trajectories were shown using lines and ribbons respectively. The posterior probability of seroconversion (i.e., $Pr(C = 1)$) is shown in the title of each panel. The observed viral load data was shown using solid dots.

## References

Deming, M. E., Dong, T. Q., Agrawal, V., Mills, M. G., Huang, M.-L. W., Greninger, A. L., Jerome, K. R., Wener, M. H., Paasche-Orlow, M. K., Kissinger, P., Luk, A., Hoffman, R. M., Stewart, J., Kottkamp, A. C., Bershteyn, A., Chu, H. Y., Stankiewicz Karita, H. C., Johnston, C. M., Wald, A., Barnabas, R., Brown, E., and Neuzil, K. (2022). Detection and kinetics of subgenomic SARS-CoV-2 RNA viral load in longitudinal diagnostic RNA positive samples. *The Journal of Infectious Diseases*, 226(5):788–796.

Gelman, A., Carlin, J. B., Stern, H. S., Dunson, D. B., Vehtari, A., and Rubin, D. B. (2013). *Bayesian data analysis, third edition*. Chapman and Hall/CRC.

Geweke, J. (1992). Evaluating the accuracy of sampling-based approaches to the calculations of posterior moments. *Bayesian statistics*, 4:641–649.

Kissler, S. M., Fauver, J. R., Mack, C., Olesen, S. W., Tai, C., Shiue, K. Y., Kalinich, C. C., Jednak, S., Ott, I. M., Vogels, C. B., et al. (2021a). Viral dynamics of acute SARS-CoV-2 infection and applications to diagnostic and public health strategies. *PLoS biology*, 19(7):e3001333.

Kissler, S. M., Fauver, J. R., Mack, C., Tai, C. G., Breban, M. I., Watkins, A. E., Samant, R. M., Anderson, D. J., Metti, J., Khullar, G., Baits, R., MacKay, M., Salgado, D., Baker, T., Dudley, J. T., Mason, C. E., Ho, D. D., Grubaugh, N. D., and Grad, Y. H. (2021b). Viral dynamics of SARS-CoV-2 variants in vaccinated and unvaccinated Persons. *New England Journal of Medicine*, 385:2489–2491.

Plummer, M. et al. (2003). JAGS: A program for analysis of Bayesian graphical models using Gibbs sampling. *Proceedings of the 3rd international workshop on distributed statistical computing*, 124(125.10):1–10.

R Core Team (2022). *R: A language and environment for statistical computing*. R Foundation for Statistical Computing, Vienna, Austria.

Stankiewicz Karita, H. C., Dong, T. Q., Johnston, C., Neuzil, K. M., Paasche-Orlow, M. K., Kissinger, P. J., Bershteyn, A., Thorpe, L. E., Deming, M., Kottkamp, A., Laufer, M., Landovitz, R. J., Luk, A., Hoffman, R., Roychoudhury, P., Magaret, C. A., Grenninger, A. L., Huang, M.-L., Jerome, K. R., Wener, M., Celum, C., Chu, H. Y., Baeten, J. M., Wald, A., Barnabas, R. V., Brown, E. R., and the Hydroxychloroquine COVID-19 PEP Study Team (2021). Trajectory of viral RNA load among persons with incident SARS-CoV-2 G614 infection (Wuhan strain) in relation to COVID-19 symptom onset and severity. *JAMA Network Open*, 5(1):e2142796.
